# Supplementary material for: No-regret Learning in Cournot Games
Source: arXiv:1906.06612 source file (2020-02-11)
Supplement: Supplementary file 1 [file appendix_results.tex]

\subsection*{More Cournot Game Examples}
In this section, we provide more examples on the learning dynamics of FKM and OMD algorithms in Cournot games with different price and cost functions. All simulations use the same hyper-parameters in Appendix A3.

We consider the following price functions:
\begin{enumerate}
\item Quadratic function: $p(y) = 1-y^2, 0\leq y \leq 1$ and $p(y) = 0, y>1$.
\item Cubic function: $p(y) = 1-y^3, 0\leq y \leq 1$ and $p(y) = 0, y>1$.
\item Exponential function: $p(y) = e-e^{y}, 0 \leq y \leq 1$ and $p(y) = 0, y>1$.
\end{enumerate}
For the cost functions, we consider linear and quadratic cost functions. All the above are just examples, and the convergence results hold for all price and cost functions if they satisfy the Assumption (A1) and (A2).

%The following plots visualize the convergence behavior of FKM and OMD in different games. 
Table~\ref{game_parameters} lists the price function, cost function and Nash equilibrium for each Cournot game example.
\begin{figure}[htbp]
	\begin{center}
		\subfigure[G1: FKM]{\includegraphics[width = 0.49\columnwidth]{appendix/FKM_case1.png}}
		\subfigure[G1: OMD]{\includegraphics[width = 0.49\columnwidth]{appendix/OMD_case1.png}}\\
		\subfigure[G2: FKM]{\includegraphics[width = 0.49\columnwidth]{appendix/FKM_case2.png}}
		\subfigure[G2: OMD]{\includegraphics[width = 0.49\columnwidth]{appendix/OMD_case2.png}}\\
		\subfigure[G3: FKM]{\includegraphics[width = 0.49\columnwidth]{appendix/FKM_case3.png}}
		\subfigure[G3: OMD]{\includegraphics[width = 0.49\columnwidth]{appendix/OMD_case3.png}}
		\caption{Dynamics of FKM and OMD in various Cournot Games.}
		\label{fig:append_case1_2_3}
	\end{center}
	\vskip -0.2in
\end{figure}
\begin{figure}[htbp]
	\ContinuedFloat
	\begin{center}
		\subfigure[G4: FKM]{\includegraphics[width = 0.49\columnwidth]{appendix/FKM_case4.png}}
		\subfigure[G4: OMD]{\includegraphics[width = 0.49\columnwidth]{appendix/OMD_case4.png}}\\
		\subfigure[G5: FKM]{\includegraphics[width = 0.49\columnwidth]{appendix/FKM_case5.png}}
		\subfigure[G5: OMD]{\includegraphics[width = 0.49\columnwidth]{appendix/OMD_case5.png}}\\
		\subfigure[G6: FKM]{\includegraphics[width = 0.49\columnwidth]{appendix/FKM_case6.png}}
		\subfigure[G6: OMD]{\includegraphics[width = 0.49\columnwidth]{appendix/OMD_case6.png}}\\
		\subfigure[G7: FKM]{\includegraphics[width = 0.49\columnwidth]{appendix/FKM_case7.png}}
		\subfigure[G7: OMD]{\includegraphics[width = 0.49\columnwidth]{appendix/OMD_case7.png}}\\
		\subfigure[G8: FKM]{\includegraphics[width = 0.49\columnwidth]{appendix/FKM_case8.png}}
		\subfigure[G8: OMD]{\includegraphics[width = 0.49\columnwidth]{appendix/OMD_case8.png}}\\
		\subfigure[G9: FKM]{\includegraphics[width = 0.49\columnwidth]{appendix/FKM_case9.png}}
		\subfigure[G9: OMD]{\includegraphics[width = 0.49\columnwidth]{appendix/OMD_case9.png}}
	\end{center}
	\vskip -0.2in
\end{figure}
%Interested readers could other price functions and individual cost functions, and as long as they satisfy (A1)-(A2), the convergence results hold.
\begin{table*}[h]
	\caption{Price, Cost Functions and NE for the Simulated Cournot Games.}
	\label{game_parameters}
	\vskip 0.15in
	\begin{center}
		\begin{small}
			\begin{sc}
				\begin{tabular}{lccc}
					\toprule
					Game Index & Price Function & Cost Function& Nash Equilibrium \\
					\midrule
					G1    & Quadratic & $C_i(x_i) = 0.05x_i, i=1,2,3,4$ & $\mathbf{x}^*=[0.199, 0.199, 0.199, 0.199]^T$\\
					G2 &  Cubic & $C_i(x_i) = 0.3x_i, i=1,2,3,4$ & $\mathbf{x}^*=[0.184, 0.184, 0.184, 0.184]^T$\\
					G3    & Exponential  &  $C_i(x_i) = 0.5x_i, i=1,2,3,4$ &  $\mathbf{x}^*=[0.162, 0.162, 0.162, 0.162]^T$\\
					G4    & Quadratic & $C_i(x_i) = 0.5x_i^2, i=1,2,3,4$ & $\mathbf{x}^*=[0.184, 0.184, 0.184, 0.184]^T$ \\
					G5     & Cubic & $C_i(x_i) = 0.5x_i^2, i=1,2,3,4$ & $\mathbf{x}^*=[0.193, 0.193, 0.193, 0.193]^T$  \\
					G6      & Exponential & $C_i(x_i) = 0.5x_i^2, i=1,2,3,4$ & $\mathbf{x}^*=[0.189, 0.189, 0.189, 0.189]^T$  \\
					G7      & Quadratic & $\begin{cases}C_1(x_1) = 0.1x_1 \\C_2(x_2) = 0.2x_2\\C_3(x_3) = 0.3 x_3\\C_4(x_4) = 0.4x_4\end{cases}$&   $\mathbf{x}^*=[0.283, 0.212, 0.141, 0.071]^T$      \\
					G8      & Cubic & $\begin{cases}C_1(x_1) = 0.1x_1 \\C_2(x_2) = 0.2x_2\\C_3(x_3) = 0.3 x_3\\C_4(x_4) = 0.4x_4\end{cases}$&   $\mathbf{x}^*=[0.276, 0.218, 0.159, 0.101]^T$      \\
					G9   & Cubic & $\begin{cases}C_1(x_1) = 0.5 x_1^2 \\C_2(x_2) = x_2^2\\C_3(x_3) = 2x_3^2\\C_4(x_4) = 4x_4^2\end{cases}$ & $\mathbf{x}^*=[0.284, 0.200, 0.126, 0.072]^T$ \\
					\bottomrule
				\end{tabular}
			\end{sc}
		\end{small}
	\end{center}
	\vskip -0.1in
\end{table*}
